# Supplementary material for: A Review of Reinforcement Learning in Financial Applications
Source: arXiv:2411.12746 source file (2024-11-01)
Supplement: Supplementary file 1 [file 0_7_appendix_only.tex]

% template.tex, dated April 5 2013
% This is a template file for Annual Reviews 1 column Journals
%
% Compilation using ar-1col-S2O.cls' - version 1.0, Aptara Inc.
% (c) 2013 AR
%
% Steps to compile: latex latex latex
%
% For tracking purposes => this is v1.0 - Apr. 2013

\documentclass{ar-1col-S2O}

\usepackage{amsfonts,amsmath,amssymb,amsthm}
\usepackage{booktabs}
\usepackage{longtable}
\usepackage{float}
\usepackage{lipsum}
\usepackage[ruled,vlined]{algorithm2e}
\usepackage{caption}
\usepackage{subcaption}
\usepackage[acronym]{glossaries}
\usepackage[backgroundcolor=white]{todonotes}
\newcommand{\todorw}[2][]{\todo[color=blue!20,size=\tiny,inline,#1]{RW: #2}}
\newcommand{\todors}[2][]
{\todo[color=yellow!20,size=\tiny,inline,#1]{RS: #2}}
\newcommand{\tododg}[2][]
{\todo[color=blue!20,size=\tiny,inline,#1]{Dale: #2}}

% \usepackage{graphicx}

% \usepackage{makecell}
\usepackage{amssymb}% http://ctan.org/pkg/amssymb
\usepackage{pifont}% http://ctan.org/pkg/pifont
\newcommand{\cmark}{\ding{51}}%
\newcommand{\xmark}{\ding{55}}%
\newcommand{\red}[1]{{\textcolor{red}{#1}}}
\newcommand{\blue}[1]{{\textcolor{blue}{#1}}}
\newcommand{\green}[1]{{\textcolor{green}{#1}}}
\newcommand{\sheng}[1]{\textcolor{yellow}{Sheng:\ #1}}
\newcommand{\yahui}[1]{\textcolor{purple}{Yahui:\ #1}}

% \usepackage[]{natbib}

% \setcitestyle{super,numbers,square}

% \usepackage{filecontents}
\usepackage{multirow}
\usepackage{tabularx}
\theoremstyle{definition}
\newtheorem{definition}{Definition}[section]

\theoremstyle{remark}
\newtheorem{remark}{Remark}

\usepackage{array} % Dale: I add this for inserting a table 

\theoremstyle{plain}
\newtheorem{thm}{Theorem}
\newtheorem{lemma}{Lemma}

\theoremstyle{definition}
\newtheorem{defin}{Definition}
\hyphenation{de-si-de-rium}

%%%%%%%%%%%%%%%%%%%%%%%%%%%%%%%%%%%%%%%%%%%%%%%%%%%%%%%%%%%%%%%%%%%%%%%%%%%%%%%%%%%%%%%%%%%%%%%%%%%%%%%%%

\usepackage[comma]{natbib}
\usepackage{url}
\setcounter{secnumdepth}{4}

% Metadata Information
\jname{Xxxx. Xxx. Xxx. Xxx.}
\jvol{AA}
\jyear{YYYY}
\doi{10.1146/((please add article doi))}


% Document starts
\begin{document}

\bibliographystyle{ar-style1.bst}
\bibliography{ref1}

% \begin{thebibliography}{00}

% \bibitem[Acevedo \& Fitzjarrald(2001)]{Acevedo:01}
% Acevedo O, Fitzjarrald D. 2001.
% The early evening surface-layer transition: temporal and spatial variability.
% \textit{J. Atmos. Sci.} 58:2650--67

% \end{thebibliography}


%%%%%%%%%%%%%%%%%%%%%%%%%%%%%%%%%%%%%%%%%%%%%%%%%%%%%%%%%%%%%%%%%%%%%%%%%%%%%%%%%%%%%%%%%%%%%%%%%%%%%%%%%%%%%%%%%%%%%%%%%%%%%%%%%%%%%%%%%%%%%%%%%%%%%%

\newpage

\appendix
\input{7_appendix}




\end{document}
